# Supplementary material for: A spatiotemporal Bayesian hierarchical model of heat-related mortality in Catalonia, Spain (2012--2022): The role of environmental and socioeconomic modifiers
Source: arXiv:2511.17148 source file (2026-10-21)
Supplement: Supplementary file 1 [file suplementary.tex]

\documentclass{article}
% Graphics and floats
\usepackage{graphicx}
\usepackage{float}
\usepackage{rotating}
\usepackage{pdflscape}

% Maths
\usepackage{amssymb}
\usepackage{amsmath}

% Tables
\usepackage{array}
\usepackage{booktabs}
\usepackage{multirow}
\usepackage{makecell}
\usepackage[table]{xcolor}
\usepackage{adjustbox}
\usepackage{caption}

% Figures with subcaptions
\usepackage{subfig}

% Define a new counter for series
\newcounter{tableseries}

% Define table numbering: S<series><letter>

% Define a new counter for series
\newcounter{figseries}

% Define table numbering: S<series><letter>

\title{Suplementary material}

\begin{document}

\section*{Suplementary Material}

% Start first series
\setcounter{tableseries}{1}  % S1
\setcounter{table}{0}        % Reset table letters

\begin{landscape}
\begin{table}[ht]
\centering
\caption{Results of the estimation of the models. Extreme maximum temperatures.}
\label{table1}
\small
\setlength{\tabcolsep}{4pt}
\adjustbox{max width=\linewidth}{
\begin{tabular}{@{}lcccccccc@{}}
\toprule

& \begin{tabular}{@{}c@{}}\textbf{RR (95\% CrI)}\end{tabular}
& \begin{tabular}{@{}c@{}}\textbf{RR (95\% CrI)}\end{tabular}
& \begin{tabular}{@{}c@{}}\textbf{RR (95\% CrI)}\end{tabular}
& \begin{tabular}{@{}c@{}}\textbf{RR (95\% CrI)}\end{tabular}
& \begin{tabular}{@{}c@{}}\textbf{RR (95\% CrI)}\end{tabular}
& \begin{tabular}{@{}c@{}}\textbf{RR (95\% CrI)}\end{tabular}
& \begin{tabular}{@{}c@{}}\textbf{RR (95\% CrI)}\end{tabular}
& \begin{tabular}{@{}c@{}}\textbf{RR (95\% CrI)}\end{tabular} \\

\midrule

$\text{Extreme heat}_{t-7}$ & & & & & & & & \\
 & 1.020 (1.004,1.037)
 & 1.019 (0.902,1.136)
 & 1.019 (1.003,1.036)
 & 1.019 (1.003,1.036)
 & 1.019 (1.002, 1.035)
 & 1.019 (1.003,1.036)
 & 1.010  (1.003,1.017)
 & 1.011 (1.003,1.018) \\

\midrule

$\text{mean(O}_{3,t-1} \ \text{to} \ \text{O}_{3,t-7})[<60.0 \mu g/m^3]$ & & & & & & & & \\
\quad $60.0~\mu\mathrm{g}/\mathrm{m}^3 \text{--} 99.9~\mu\mathrm{g}/\mathrm{m}^3$
&  
& 1.012 (0.999,1.026)
&  
&  
&  
&  
&  
&  \\

\quad $100.0~\mu\mathrm{g}/\mathrm{m}^3 \text{--} 119.9~\mu\mathrm{g}/\mathrm{m}^3$
&  
& 1.081 (0.999,1.169)
&  
&  
&  
&  
&  
&  \\

\quad $\ge 120.0~\mu\mathrm{g}/\mathrm{m}^3$
&  
& 1.325 (1.069,1.581)
&  
&  
&  
&  
&  
&  \\

\midrule

$\text{mean(NO}_{2,t-1} \ \text{to} \ \text{NO}_{2,t-7})[<10.0 \mu g/m^3]$ & & & & & & \\
\quad $10.0~\mu\mathrm{g}/\mathrm{m}^3 \text{--} 24.9~\mu\mathrm{g}/\mathrm{m}^3$
&  
&  
&  0.997 (0.987,1.007)
&  
&  
&  
&  
&  \\

\quad $\ge 25.0~\mu\mathrm{g}/\mathrm{m}^3$
&  
& 
&  1.017 (0.994,1.041)
&  
&  
&  
&  
&  \\
\midrule

$\text{mean(PM}_{10,t-1} \ \text{to} \ \text{PM}_{10,t-7})[<15.0 \mu g/m^3]$ & & & & & & \\
\quad $15.0~\mu\mathrm{g}/\mathrm{m}^3 \text{--} 44.9~\mu\mathrm{g}/\mathrm{m}^3$
&  
& 
&  
&  1.002 (0.993,1.011)
&  
&  
&  
&  \\

\quad $\ge 45.0~\mu\mathrm{g}/\mathrm{m}^3$
&  
& 
&  
&  1.046 (0.905,1.208)
&  
&  
&  
&  \\

\midrule

$\text{Q4 relative humidity}_{t-7} \text{[No]}$ & & & & & & \\
&  
& 
&  
&  
&  0.997 (0.988,1.006)
&  
&  
&  \\

\midrule

$\text{Average net income per person}[<11,490.7~\text{€}]$ & & & & & & \\
\quad 11,490.7~\text{€} \text{--} 12,893.5~\text{€}
&  
& 
&  
&  
&  
&  1.006 (0.976,1.037)
&  
&  \\

\quad 12,893.6~\text{€} \text{--} 14,650.2~\text{€}
&  
& 
&  
&  
&  
&  1.005 (0.966,1.047)
&  
&  \\

\quad $> 14,650.2~\text{€}$
&  
& 
&  
&  
&  
&  0.977 (0.928,1.028)
&  
&  \\

\midrule

$\text{Gini index}[<28.3]$ & & & & & & \\
\quad 28.3 \text{--} 30.1
&  
& 
&  
&  
&  
&  
&  1.048 (1.022,1.074)
&  \\

\quad 30.2 \text{--} 32.4
&  
& 
&  
&  
&  
&  
&  1.071 (1.040,1.103)
&  \\

\quad $>32.4$
&  
& 
&  
&  
&  
&  
&  1.050 (1.022,1.098)
&  \\

\midrule

$\text{Population aged 65 or over}(<16.6\%)$ & & & & & & \\
\quad 16.6\% \text{--} 18.6\%
&  
& 
&  
&  
&  
&  
&  
& 1.054 (1.025,1.084)\\

\quad 18.7\% \text{--} 21.3\%
&  
& 
& 
&  
&  
&  
&  
& 1.140 (1.103,1.179) \\

\quad $>21.3\%$
&  
& 
&  
&  
&  
&  
&  
& 1.054 (1.025,1.084) \\

\bottomrule
\end{tabular}
}
{\raggedright\small
\textbf{RR}: Relative risk. \textbf{95\% CrI}: 95\% credibility interval. \textbf{Reference category in brackets}. Adjusted for individual heterogeneity (ABS); seasonality (month); trend (year); and spatial dependence. Population of the ABS offset.
\par
}
\end{table}
\end{landscape}

\begin{landscape}
\begin{table}[ht]
\centering
\caption{Results of the estimation of the models. Heatwaves.}
\label{table2}
\small
\setlength{\tabcolsep}{4pt}
\adjustbox{max width=\linewidth}{
\begin{tabular}{@{}lcccccccc@{}}
\toprule

& \begin{tabular}{@{}c@{}}\textbf{RR (95\% CrI)}\end{tabular}
& \begin{tabular}{@{}c@{}}\textbf{RR (95\% CrI)}\end{tabular}
& \begin{tabular}{@{}c@{}}\textbf{RR (95\% CrI)}\end{tabular}
& \begin{tabular}{@{}c@{}}\textbf{RR (95\% CrI)}\end{tabular}
& \begin{tabular}{@{}c@{}}\textbf{RR (95\% CrI)}\end{tabular}
& \begin{tabular}{@{}c@{}}\textbf{RR (95\% CrI)}\end{tabular}
& \begin{tabular}{@{}c@{}}\textbf{RR (95\% CrI)}\end{tabular}
& \begin{tabular}{@{}c@{}}\textbf{RR (95\% CrI)}\end{tabular} \\

\midrule

$\text{Extreme heat}_{t-7}$ & & & & & & & & \\
 & 1.019 (1.003,1.035)
 & 1.019 (0.973,1.065)
 & 1.019 (1.004,1.034)
 & 1.019 (1.004,1.035)
 & 1.020 (1.004,1.036)
 & 1.016 (1.004,1.028)
 & 1.016 (1.004,1.028)
 & 1.016 (1.004,1.028) \\

\midrule

$\text{mean(O}_{3,t-1} \ \text{to} \ \text{O}_{3,t-7})[<60.0 \mu g/m^3]$ & & & & & & & & \\
\quad $60.0~\mu\mathrm{g}/\mathrm{m}^3 \text{--} 99.9~\mu\mathrm{g}/\mathrm{m}^3$
&  
& 1.012 (0.998,1.026)
&  
&  
&  
&  
&  
&  \\

\quad $100.0~\mu\mathrm{g}/\mathrm{m}^3 \text{--} 119.9~\mu\mathrm{g}/\mathrm{m}^3$
&  
& 1.072 (0.991,1.160)
&  
&  
&  
&  
&  
&  \\

\quad $\ge 120.0~\mu\mathrm{g}/\mathrm{m}^3$
&  
& 1.297 (0.948,1.773)
&  
&  
&  
&  
&  
&  \\

\midrule

$\text{mean(NO}_{2,t-1} \ \text{to} \ \text{NO}_{2,t-7})[<10.0 \mu g/m^3]$ & & & & & & \\
\quad $10.0~\mu\mathrm{g}/\mathrm{m}^3 \text{--} 24.9~\mu\mathrm{g}/\mathrm{m}^3$
&  
&  
&  0.996 (0.987,1.005)
&  
&  
&  
&  
&  \\

\quad $\ge 25.0~\mu\mathrm{g}/\mathrm{m}^3$
&  
& 
&  1.012 (0.990,1.033)
&  
&  
&  
&  
&  \\
\midrule

$\text{mean(PM}_{10,t-1} \ \text{to} \ \text{PM}_{10,t-7})[<15.0 \mu g/m^3]$ & & & & & & \\
\quad $15.0~\mu\mathrm{g}/\mathrm{m}^3 \text{--} 44.9~\mu\mathrm{g}/\mathrm{m}^3$
&  
& 
&  
&  0.999 (0.991,1.008)
&  
&  
&  
&  \\

\quad $\ge 45.0~\mu\mathrm{g}/\mathrm{m}^3$
&  
& 
&  
&  1.018 (0.939,1.103)
&  
&  
&  
&  \\

\midrule

$\text{Q4 relative humidity}_{t-7} \text{[No]}$ & & & & & & \\
&  
& 
&  
&  
&  0.999 (0.990,1.008)
&  
&  
&  \\

\midrule

$\text{Average net income per person}[<11,490.7~\text{€}]$ & & & & & & \\
\quad 11,490.7~\text{€} \text{--} 12,893.5~\text{€}
&  
& 
&  
&  
&  
&  1.006 (0.976,1.037)
&  
&  \\

\quad 12,893.6~\text{€} \text{--} 14,650.2~\text{€}
&  
& 
&  
&  
&  
&  1.005 (0.965,1.046)
&  
&  \\

\quad $> 14,650.2~\text{€}$
&  
& 
&  
&  
&  
&  0.976 (0.928,1.026)
&  
&  \\

\midrule

$\text{Gini index}[<28.3]$ & & & & & & \\
\quad 28.3 \text{--} 30.1
&  
& 
&  
&  
&  
&  
&  1.047 (1.022,1.073)
&  \\

\quad 30.2 \text{--} 32.4
&  
& 
&  
&  
&  
&  
&  1.070 (1.039,1.102)
&  \\

\quad $>32.4$
&  
& 
&  
&  
&  
&  
&  1.058 (1.021,1.097)
&  \\

\midrule

$\text{Population aged 65 or over}(<16.6\%)$ & & & & & & \\
\quad 16.6\% \text{--} 18.6\%
&  
& 
&  
&  
&  
&  
&  
& 1.048 (1.018,1.079)\\

\quad 18.7\% \text{--} 21.3\%
&  
& 
& 
&  
&  
&  
&  
& 1.127 (1.089,1.166) \\

\quad $>21.3\%$
&  
& 
&  
&  
&  
&  
&  
& 1.154 (1.106,1.203) \\

\bottomrule
\end{tabular}
}
{\raggedright\small
\textbf{RR}: Relative risk. \textbf{95\% CrI}: 95\% credibility interval. \textbf{Reference category in brackets}. Adjusted for individual heterogeneity (ABS); seasonality (month); trend (year); and spatial dependence. Population of the ABS offset.
\par
}
\end{table}
\end{landscape}

% Start second series
\stepcounter{tableseries}    % S2
\setcounter{table}{0}        % Reset letter counter

\begin{landscape} 
\begin{table}[ht]
\centering
\caption{Descriptive statistics on mortality. Total mortality and causes with more than 3\% of deaths. Catalonia, summers of 2012-2022.}
\label{table3}
\small
\setlength{\tabcolsep}{4pt}
\adjustbox{max width=\linewidth}{
\begin{tabular}{@{}lccccccccccc@{}}
\toprule

& \begin{tabular}{@{}c@{}}\textbf{Total}\end{tabular}
& \begin{tabular}{@{}c@{}}\textbf{Tumors}\end{tabular}
& \begin{tabular}{@{}c@{}}\textbf{Circulatory} \\ \textbf{diseases}\end{tabular}
& \begin{tabular}{@{}c@{}}\textbf{Respiratory} \\ \textbf{diseases} \end{tabular}
& \begin{tabular}{@{}c@{}}\textbf{Nervous system} \\  \textbf{diseases} \end{tabular}
& \begin{tabular}{@{}c@{}}\textbf{Mental} \\ \textbf{diseases} \end{tabular}
& \begin{tabular}{@{}c@{}}\textbf{Digestive} \\ \textbf{disorders} \end{tabular}
& \begin{tabular}{@{}c@{}}\textbf{External causes}\\ \textbf{of mortality} \end{tabular}
& \begin{tabular}{@{}c@{}}\textbf{Genitourinary} \\ \textbf{diseases}\end{tabular}
& \begin{tabular}{@{}c@{}}\textbf{Endocrine and} \\ \textbf{metabolic} \\ \textbf{diseases}\end{tabular} \\

\midrule

\textbf{Sex, n=216989} & & & & & & & & & & \\

\quad Female 
& 108315 (49.92\%)
& 25271 (40.42\%) 
& 29712 (53.85\%) 
& 7411 (41.79\%)
& 9905 (62.79\%) 
& 9569 (66.67\%) 
& 5273 (49.49\%) 
& 4087 (39.66\%) 
& 4076 (57.62\%)  
& 3955 (57.01\%)  \\

\quad Male 
& 108674 (50.08\%) 
& 37244 (59.58\%)
& 25467 (46.15\%) 
& 10321 (58.21\%) 
& 5871 (37.21\%) 
& 4784 (33.33\%) 
& 5381 (50.51\%) 
& 6219 (60.34\%)
& 2998 (42.38\%) 
& 2982 (42.99\%) \\
\midrule

\textbf{Age, n=216989} & & & & & & & & & & \\

& 79.38 (14.68)
& 73.77 (13.45) 
& 82.51 (12.35) 
& 82.88 (11.57) 
& 82.72 (11.82) 
& 87.93 (7.94)
& 78.66 (13.86) 
& 68.52 (22.98)
& 86.1 (8.98) 
& 82.45 (12.72) \\

& 83 [73, 89] 
& 76 [65, 84] 
& 86 [77, 91] 
& 85 [78, 90] 
& 85 [79, 90] 
& 89 [84, 93] 
& 82 [71, 89] 
& 76 [50, 87] 
& 88 [82, 92] 
& 85 [78, 90]  \\

\midrule

\textbf{Children, n=592} & & & & & & & & & & \\

\quad Under one month old 
& 421 (71.11\%)
& 2 (40\%) 
& 1 (12.5\%) 
& 
& 5 (23.81\%) 
& 
& 1 (25\%)
& 3 (21.43\%) 
& 1 (50\%)
& 10 (38.46\%)   \\

\quad Under one year old 
& 171 (28.89\%) 
& 3 (60\%) 
& 7 (87.5\%) 
& 4 (100\%) 
& 16 (76.19\%) 
& 
& 3 (75\%) 
& 11 (78.57\%) 
& 1 (50\%)
& 16 (61.54\%) \\

\midrule

\textbf{Marital Status, n=152681} & & & & & & & & & & \\

\quad Divorced 
& 7395 (4.84\%)
& 2881 (6.36\%)
& 1683 (4.24\%)
& 556 (4.27\%)
& 340 (2.97\%)
& 201 (1.92\%)
& 530 (7.02\%)
& 548 (7.45\%)
& 118 (2.55\%)
& 185 (3.89\%) \\

\quad Married 
& 64376 (42.16\%)
& 25710 (56.74\%)
& 14646 (36.87\%)
& 5311 (40.82\%)
& 4368 (38.15\%)
& 2836 (27.16\%)
& 2960 (39.23\%)
& 2668 (36.27\%)
& 1500 (32.44\%)
& 1725 (36.24\%) \\

\quad Single 
& 16985 (11.12\%)
& 4479 (9.88\%)
& 3941 (9.92\%)
& 1330 (10.22\%)
& 1067 (9.32\%)
& 1066 (10.21\%)
& 901 (11.94\%)
& 1719 (23.37\%)
& 427 (9.23\%)
& 482 (10.13\%) \\

\quad Widower/Widow 
& 63925 (41.87\%)
& 12244 (27.02\%)
& 19458 (48.98\%)
& 5814 (44.69\%)
& 5675 (49.56\%)
& 6339 (60.71\%)
& 3154 (41.8\%)
& 2420 (32.9\%)
& 2579 (55.77\%)
& 2368 (49.75\%) \\
\midrule

\textbf{Studies, n=212403} & & & & & & & & & & \\

\quad Insufficient instruction 
& 45030 (21.2\%)
& 9161 (14.9\%)
& 12714 (23.42\%)
& 4398 (25.19\%)
& 3741 (24.1\%)
& 4211 (29.72\%)
& 2313 (22.17\%)
& 1587 (16.38\%)
& 1802 (25.78\%)
& 1732 (25.43\%) \\

\quad Primary 
& 122930 (57.88\%)
& 34893 (56.77\%)
& 31683 (58.36\%)
& 10211 (58.49\%)
& 9134 (58.83\%)
& 8148 (57.5\%)
& 6081 (58.3\%)
& 5280 (54.51\%)
& 4179 (59.79\%)
& 4057 (59.57\%) \\

\quad Secondary 
& 22255 (10.48\%)
& 8443 (13.74\%)
& 4986 (9.18\%)
& 1430 (8.19\%)
& 1322 (8.51\%)
& 940 (6.63\%)
& 1093 (10.48\%)
& 1465 (15.12\%)
& 508 (7.27\%)
& 544 (7.99\%) \\

\quad University 
& 16499 (7.77\%)
& 6620 (10.77\%)
& 3733 (6.88\%)
& 1059 (6.07\%)
& 993 (6.4\%)
& 671 (4.74\%)
& 683 (6.55\%)
& 942 (9.72\%)
& 382 (5.47\%)
& 347 (5.1\%) \\

\quad Vocational training 
& 5689 (2.68\%)
& 2346 (3.82\%)
& 1173 (2.16\%)
& 361 (2.07\%)
& 336 (2.16\%)
& 201 (1.42\%)
& 261 (2.5\%)
& 413 (4.26\%)
& 118 (1.69\%)
& 130 (1.91\%) \\
\midrule

\textbf{Occupation, n=164291} & & & & & & & & & & \\

\quad Occupied 
& 7534 (4.59\%)
& 3775 (8.17\%)
& 1466 (3.53\%)
& 231 (1.69\%)
& 144 (1.2\%)
& 48 (0.43\%)
& 265 (3.32\%)
& 1063 (15.05\%)
& 34 (0.59\%)
& 95 (1.71\%) \\

\quad Other 
& 33261 (20.25\%)
& 6797 (14.7\%)
& 9047 (21.77\%)
& 2527 (18.52\%)
& 2941 (24.44\%)
& 2938 (26.36\%)
& 1675 (20.97\%)
& 1464 (20.72\%)
& 1379 (24.08\%)
& 1306 (23.51\%) \\

\quad Pensioner 
& 112829 (68.68\%)
& 31290 (67.69\%)
& 29014 (69.83\%)
& 10280 (75.32\%)
& 8392 (69.75\%)
& 7867 (70.59\%)
& 5355 (67.05\%)
& 3668 (51.93\%)
& 4106 (71.71\%)
& 3888 (69.98\%) \\

\quad Permanent inactivity 
& 7854 (4.78\%)
& 3169 (6.86\%)
& 1486 (3.58\%)
& 505 (3.7\%)
& 500 (4.16\%)
& 277 (2.49\%)
& 466 (5.83\%)
& 442 (6.26\%)
& 186 (3.25\%)
& 225 (4.05\%) \\

\quad Student 
& 304 (0.19\%)
& 79 (0.17\%)
& 19 (0.05\%)
& 8 (0.06\%)
& 25 (0.21\%)
& 
& 8 (0.1\%)
& 123 (1.74\%)
& 4 (0.07\%)
& 8 (0.14\%) \\

\quad Unemployed 
& 2509 (1.53\%)
& 1118 (2.42\%)
& 519 (1.25\%)
& 97 (0.71\%)
& 30 (0.25\%)
& 15 (0.13\%)
& 218 (2.73\%)
& 304 (4.3\%)
& 17 (0.3\%)
& 34 (0.61\%) \\
\midrule

\textbf{Total}
& 216989 (100\%)
& 62515 (28.81\%) 
& 55179 (25.43\%) 
& 17732 (8.17\%)
& 15776 (7.27\%) 
& 14353 (6.61\%)
& 10654 (4.91\%) 
& 10306 (4.75\%) 
& 7074 (3.26\%) 
& 6937 (3.2\%) \\

\bottomrule
\end{tabular}
}
\end{table}
\end{landscape}

\begin{landscape}
\begin{table}[ht]
\centering
\caption{Descriptive statistics on mortality. Causes with less than 3\% of deaths. Catalonia, summers of 2012-2022.}
\label{table4}
\small
\setlength{\tabcolsep}{4pt}
\adjustbox{max width=\linewidth}{
\begin{tabular}{@{}lcccccccccc@{}}
\toprule

& \begin{tabular}{@{}c@{}}\textbf{COVID-19}\end{tabular}
& \begin{tabular}{@{}c@{}}\textbf{Symptoms and} \\ \textbf{abnormal findings}\end{tabular}
& \begin{tabular}{@{}c@{}}\textbf{Infectious} \\ \textbf{diseases}\end{tabular}
& \begin{tabular}{@{}c@{}}\textbf{Musculoskeletal} \\ \textbf{diseases}\end{tabular}
& \begin{tabular}{@{}c@{}}\textbf{Hematological and} \\ \textbf{immune diseases}\end{tabular}
& \begin{tabular}{@{}c@{}}\textbf{Skin} \\ \textbf{diseases}\end{tabular}
& \begin{tabular}{@{}c@{}}\textbf{Congenital} \\ \textbf{malformations}\end{tabular}
& \begin{tabular}{@{}c@{}}\textbf{Perinatal} \\ \textbf{conditions}\end{tabular}
& \begin{tabular}{@{}c@{}}\textbf{Pregnancy and} \\ \textbf{childbirth}\end{tabular} \\

\midrule

\textbf{Sex, n=216989} & & & & & & & & & & \\

\quad Female 
& 1933 (47.58\%)
& 2045 (53.84\%)
& 1806 (52.48\%)
& 1914 (70.86\%)
& 582 (54.91\%)
& 437 (66.92\%)
& 196 (49.12\%)
& 138 (40.23\%)
& 5 (100\%) \\

\quad Male 
& 2130 (52.42\%)
& 1753 (46.16\%)
& 1635 (47.52\%)
& 787 (29.14\%)
& 478 (45.09\%)
& 216 (33.08\%)
& 203 (50.88\%)
& 205 (59.77\%)
&  \\
\midrule

\textbf{Age, n= 216989} & & & & & & & & & & \\
& 82.85 (11.86)
& 79.32 (18.7)  
& 77.99 (15.47)
& 86.54 (10.35) 
& 81.67 (15.53)
& 85.73 (10.13)
& 38.51 (32.69) 
& 0.72 (5.56)
& 40.4 (6.77)  \\

& 86 [77, 91]
& 85 [71, 92]
& 82 [72, 89]
& 89 [83, 93] 
& 86 [77, 91] 
& 87 [82, 92] 
& 47 [0, 64] 
& 0 [0, 0] 
& 42 [41, 43]\\
\midrule

\textbf{Children, n= 592} & & & & & & & & & & \\
\quad Under one month old 
& 
& 8 (19.51\%)
& 3 (42.86\%)
& 
& 
& 
& 78 (63.41\%)
& 309 (92.24\%)
& 0 (0\%)\\

\quad Under one year old
& 
& 33 (80.49\%)
& 4 (57.14\%)
&
& 2 (100\%)
& 
& 45 (36.59\%)
& 26 (7.76\%)
& \\

\midrule

\textbf{Marital Status, n= 152681} & & & & & & & & & &  \\

\quad Divorced
&
& 123 (5.12\%)
& 135 (5.28\%)
& 50 (2.88\%)
& 29 (3.83\%)
& 14 (3.21\%)
& 2 (0.69\%)
& 
&  \\

\quad Married
& 
& 776 (32.28\%)
& 958 (37.44\%)
& 499 (28.78\%)
& 259 (34.17\%)
& 114 (26.15\%)
& 42 (14.43\%)
& 266 (100\%)
& 4 (100\%) \\

\quad Single 
& 
& 378 (15.72\%)
& 395 (15.44\%)
& 184 (10.61\%)
& 95 (12.53\%)
& 37 (8.49\%)
& 218 (74.91\%)
&  
& \\

\quad Widower/Widow
&  
& 1127 (46.88\%)
& 1071 (41.85\%)
& 1001 (57.73\%)
& 375 (49.47\%)
& 271 (62.16\%)
& 29 (9.97\%)
&  
&  \\
\midrule

\textbf{Studies, n= 212403} & & & & & & & & & & \\

\quad Insufficient instruction 
& 797 (19.91\%)
& 717 (19.68\%)
& 749 (22.45\%)
& 638 (23.94\%)
& 231 (22.38\%)
& 164 (25.51\%)
& 71 (29.34\%)
& 4 (66.67\%) 
&  \\

\quad Primary 
& 2338 (58.39\%)
& 2242 (61.53\%)
& 1949 (58.41\%)
& 1596 (59.89\%)
& 614 (59.5\%)
& 393 (61.12\%)
& 128 (52.89\%)
& 2 (33.33\%)
& 2 (40\%) \\

\quad Secondary 
& 426 (10.64\%)
& 362 (9.93\%)
& 335 (10.04\%)
& 235 (8.82\%)
& 96 (9.3\%)
& 45 (7\%)
& 24 (9.92\%)
&  
& 1 (20\%) \\

\quad University 
& 330 (8.24\%)
& 238 (6.53\%)
& 226 (6.77\%)
& 158 (5.93\%)
& 72 (6.98\%)
& 32 (4.98\%)
& 11 (4.55\%)
&  
& 2 (40\%) \\

\quad Vocational training 
& 113 (2.82\%)
& 85 (2.33\%)
& 78 (2.34\%)
& 38 (1.43\%)
& 19 (1.84\%)
& 9 (1.4\%)
& 8 (3.31\%)
&  
&  \\
\midrule

\textbf{Occupation, n=164291} & & & & & & & & & & \\

\quad Occupied 
& 139 (3.47\%)
& 140 (4.78\%)
& 72 (2.87\%)
& 23 (0.99\%)
& 23 (2.98\%)
& 2 (0.38\%)
& 11 (4.87\%)
&  
& 3 (100\%)\\

\quad Other 
& 821 (20.49\%)
& 691 (23.62\%)
& 538 (21.44\%)
& 636 (27.3\%)
& 155 (20.1\%)
& 162 (30.51\%)
& 132 (58.41\%)
& 52 (100\%)
&  \\

\quad Pensioner 
& 2852 (71.19\%)
& 1890 (64.59\%)
& 1702 (67.84\%)
& 1586 (68.07\%)
& 547 (70.95\%)
& 338 (63.65\%)
& 54 (23.89\%)
&  
&  \\

\quad Permanent inactivity 
& 144 (3.59\%)
& 150 (5.13\%)
& 149 (5.94\%)
& 74 (3.18\%)
& 32 (4.15\%)
& 29 (5.46\%)
& 20 (8.85\%)
&  
&  \\

\quad Student 
& 1 (0.02\%)
& 6 (0.21\%)
& 9 (0.36\%)
& 1 (0.04\%)
& 4 (0.52\%)
&  
& 9 (3.98\%)
&
&  \\

\quad Unemployed 
& 49 (1.22\%)
& 49 (1.67\%)
& 39 (1.55\%)
& 10 (0.43\%)
& 10 (1.3\%)
& 
& 
&  
&  \\
\midrule

Total 
& 4063 (1.87\%)
& 3798 (1.75\%)
& 3441 (1.59\%) 
& 2701 (1.24\%) 
& 1060 (0.49\%) 
& 653 (0.3\%)
& 399 (0.18\%)
& 343 (0.16\%)
& 5 (0\%) \\

\bottomrule
\end{tabular}
}
\end{table}
\end{landscape}

\stepcounter{figseries}

\begin{landscape}
\begin{figure}[H] 
\centering 
\caption{Temporal evolution of the median of the minimum temperature in 2012-2021 and 2022.} 

\includegraphics[width=0.72\linewidth]{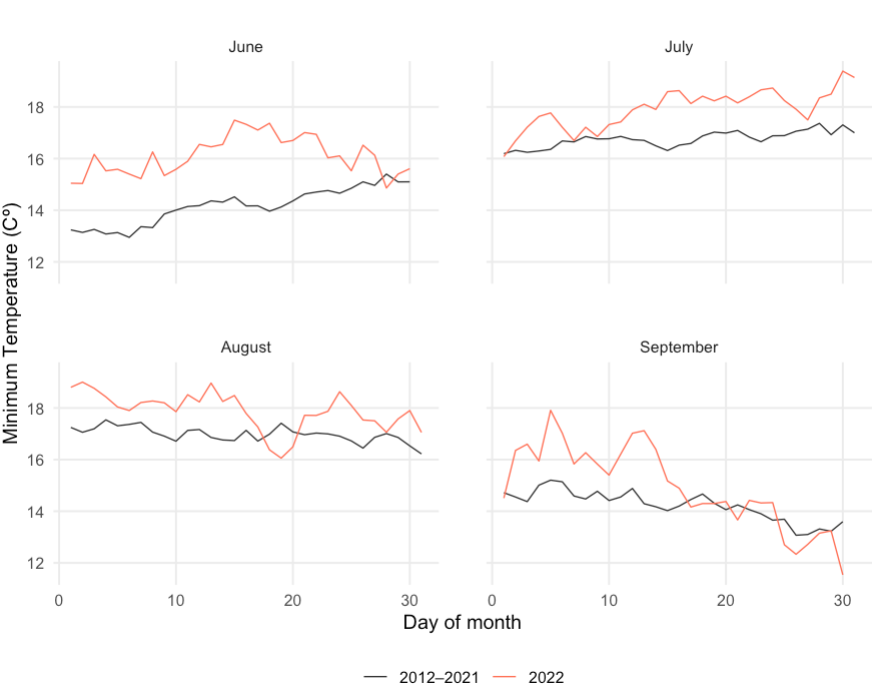}

\label{fig1}
\end{figure}
\end{landscape}

\stepcounter{figseries}

\begin{landscape}
\begin{figure}[H] 
\centering 
\caption{Temporal evolution of the median of the relative humidity in 2012-2021 and 2022.} 

\includegraphics[width=0.72\linewidth]{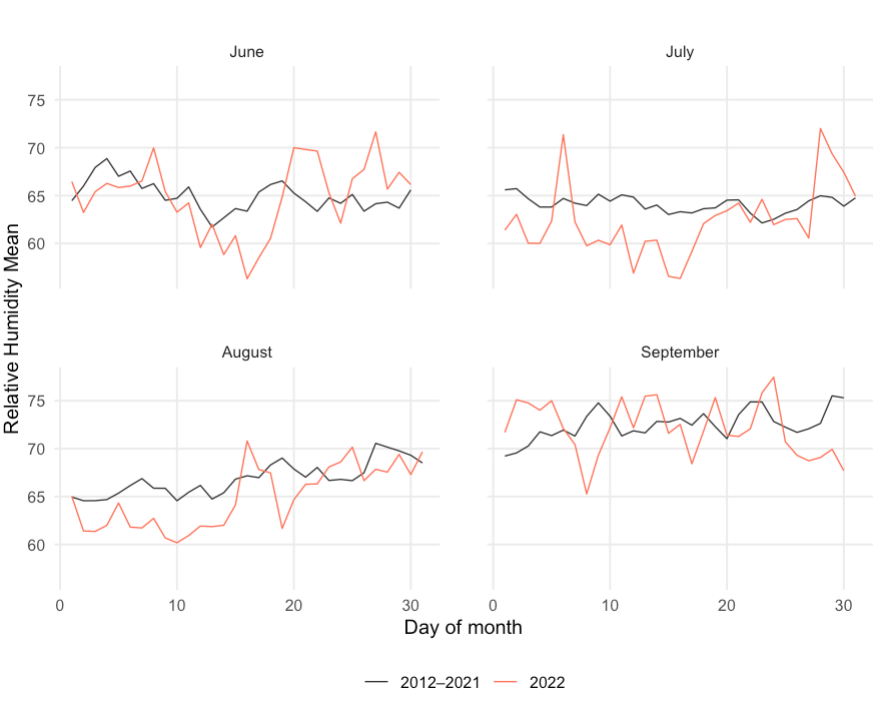}

\label{fig2}
\end{figure}
\end{landscape}

\stepcounter{figseries}

\begin{landscape}
\begin{figure}[H] 
\centering 
\caption{Temporal evolution of the median of PM10 in 2012-2021 and 2022.} 

\includegraphics[width=0.72\linewidth]{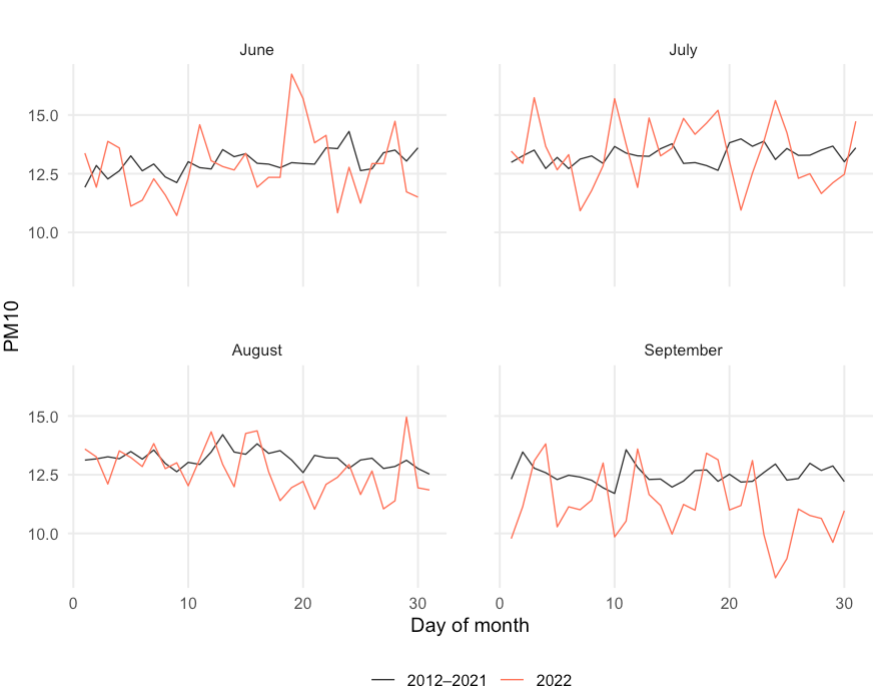}

\label{fig3}
\end{figure}
\end{landscape}

\stepcounter{figseries}

\begin{landscape}
\begin{figure}[H] 
\centering 
\caption{Temporal evolution of the median of NO2 in 2012-2021 and 2022.} 

\includegraphics[width=0.72\linewidth]{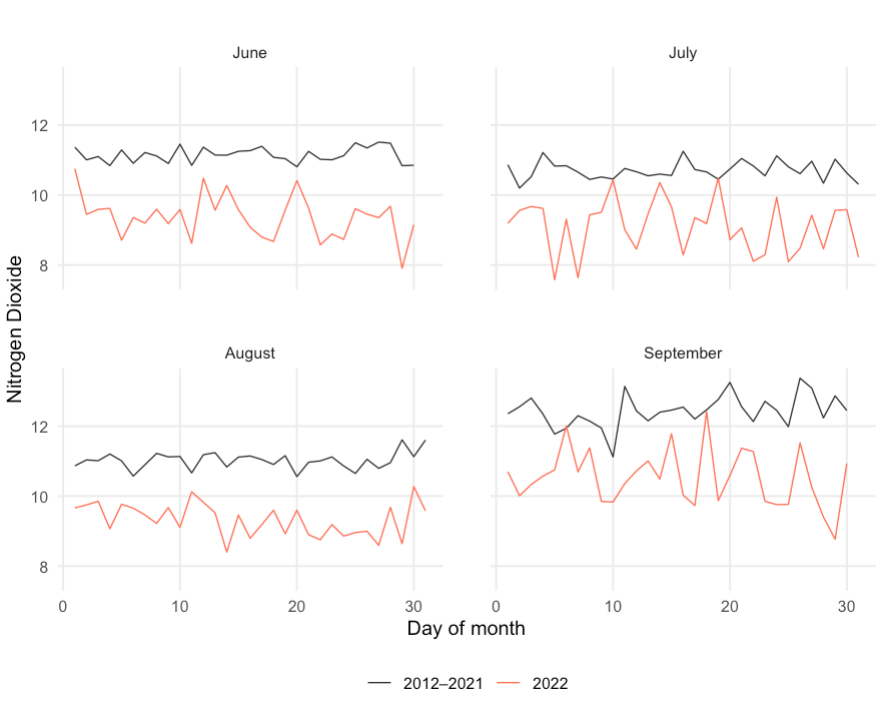}

\label{fig4}
\end{figure}
\end{landscape}

\end{document}
